# Supplementary material for: Large-scale Reinforcement Learning for Diffusion Models
Source: arXiv:2401.12244 source file (2024-01-20)
Supplement: Supplementary file 1 [file appendix.tex]

% Training Reward curve
\section{Appendix}

% Visualization of our results compared to base SD2 model
\begin{figure*}[t]
  \centering
  % \fbox{\rule{0pt}{2in} \rule{0.8\linewidth}{0pt}}
   % \includegraphics[width=0.8\linewidth]
   \includegraphics[width=\linewidth]{figures/sd2_ours_6_truncatetext.pdf}

   \caption{\textbf{Effect of RL Finetuning.} Comparison of samples (using the same random seed) from original SD2 model and our RL-fine-tuned model.}
   \label{fig:sd2_ours_6}
\end{figure*}

% Effect of pretraining dataset
\begin{figure}[!tb]
  \centering
   \includegraphics[width=\linewidth]{figures/pretraining_effect_4imgs.pdf}
   \caption{\textbf{Effect of pretraining loss.} The images are sampled using the same random seeds from the models trained without and with pre-training loss, after the same number of iterations. Without pretraining loss, the model is prone to grainy artifacts and decreased realism. }
   \label{fig:pretraining_effect}
\end{figure}

% Human Eval on skintone & compositionality 

\begin{figure}[t]{\textwidth}
\centering
   \includegraphics[width=\linewidth]{figures/eval_on_skintone_compositionality.pdf}
  \caption{Human Eval Results on skintone diversity and compositionality}
  \label{fig:skintone_compositionality_eval}
\end{figure}
